# Supplementary material for: Is It Bad to Work All the Time? Cross-Cultural Evaluation of Social Norm Biases in GPT-4
Source: arXiv:2505.18322 source file (2025-05-23)
Supplement: Supplementary file 1 [file app_evaluation_dataset.tex]

In our final dataset after the evaluation of RoTs, each example represents a social norm RoT, along with a rich set of annotations. For each norm, we record the country or culture it is associated with (e.g., China, India, Iran, U.S.) and whether it was written by a human, a language model without cultural guidance, or a model prompted to reflect a specific culture. Human annotators evaluate each norm for accuracy, cultural specificity, and whether it reflects a stereotype. 

In addition to human ratings, we generate model-predicted accuracy scores for each norm using both a default prompt and prompts framed by specific cultural contexts. These predictions allow us to compare how the model's behavior changes across cultures. 

Specifically, We define our dataset as a collection of annotated social norms:

\begin{equation}
D = \{ d_i \}_{i=1}^{N}
\end{equation}

Each data point \( d_i \) contains the following information:

\begin{equation}
\begin{aligned}
d_i = (&r_i, c_i, s_i, \text{accuracy}_i, \text{culture}_i, \text{stereotype}_i, \\
      &a_i, \phi^{\text{default}}_i, \phi^{\text{China}}_i, \phi^{\text{India}}_i, \phi^{\text{Iran}}_i, \phi^{\text{US}}_i)
\end{aligned}
\end{equation}

\begin{itemize}
    \item \( r_i \): the \(i\)-th social norm (Rule of Thumb).
    \item \( c_i \): the associated culture label (China, India, Iran, U.S.).
    \item \( s_i \): the source of the norm (human-written, GPT, or GPT with cultural prompt).
    \item \( \text{accuracy}_i \in [1, 5] \): the human-rated accuracy score.
    \item \( \text{culture}_i \in [1, 5] \): the human-rated culture-specificity score.
    \item \( \text{stereotype}_i \in \{0, 1\} \): whether the norm was judged as stereotypical.
    \item \( a_i \): the annotator id.
    \item \( \phi^{\text{default}}_i \): a set of 30 model-predicted accuracy scores under the default prompt.
    \item \( \phi^c_i \): model-predicted accuracy scores under the culture-specific prompt for culture \( c \in \{\text{China, India, Iran, U.S.}\} \).
\end{itemize}
