# Supplementary material for: Is It Bad to Work All the Time? Cross-Cultural Evaluation of Social Norm Biases in GPT-4
Source: arXiv:2505.18322 source file (2025-05-23)
Supplement: Supplementary file 2 [file app_guideline_collecting.tex]

\subsection*{Part 1. \textbf{Answer the following questions.} If unsure, provide the most likely answer.}
\begin{tightitemize}
    \item Which country does this flag represent?
    \item What is the name of this figure?
    \item What is this place?
    \item What are the people doing? Use 1--2 sentences to describe what they are making.
    \item What is this festival? Describe your experience with it in 2--3 sentences.
\end{tightitemize}

\subsection*{Part 2. \textbf{Write Rules-of-Thumb to explain social norms in Iran \iran{} to a computer!}}

Your task is to write social norms \textbf{Rules-of-Thumb (RoTs)} inspired by the story at the bottom. We want RoTs that explain what we consider good and bad behavior.

You can think of the computer like a five-year-old child who doesn't know how the world works. We have to explain the basics to them about what people think is right and wrong in society, and how our actions make other people feel.

\subsubsection*{Requirements for writing RoTs:}
\begin{itemize}
    \item \textbf{Iran-Culture-Driven}: RoTs should align with established norms and practices in Iran.
    \item \textbf{Judgement + Action}: Each RoT should follow the format: \textit{It is [the judgment] to [the action]}. \\
    Example: \textit{It is rude to curse at people.}
    \item \textbf{Verb-Centric}: Anchor each RoT to a specific verb from the story (tense doesn't matter). \\
    Examples:
    \begin{itemize}
        \item \textbf{curse} $\rightarrow$ \textit{It is rude to curse at people.}
        \item \textbf{liking} $\rightarrow$ \textit{It's good to like your relatives.}
        \item \textbf{invite} $\rightarrow$ \textit{It’s devastating to be excluded from a wedding you were invited to.}
    \end{itemize}
    \item \textbf{Specificity}: Avoid overly generic statements.
    \item \textbf{Quantity}: Write \textbf{3 to 5 RoTs}.
\end{itemize}

\subsubsection*{Bad Examples and Corrections:}
\begin{itemize}
    \item \textbf{Bad RoT:} \textit{curse $\rightarrow$ Cursing at people is rude.} \\
    \textbf{Reason:} Does not follow the structure "It is [the judgment] to [the action]". \\
    \textbf{Correction:} \textit{It is rude to curse at people.}
    
    \item \textbf{Bad RoT:} \textit{sleep $\rightarrow$ Studies have shown people perform best on exams after sleeping at least seven hours.} \\
    \textbf{Reason:} Too encyclopedic. RoTs should reflect everyday, commonsense norms. \\
    \textbf{Correction:} \textit{It is ok to sleep for seven hours before exams.}

    \item \textbf{Bad RoT:} \textit{cut $\rightarrow$ It's cold to cut off contact with Jimmy.} \\
    \textbf{Reason:} Should be understandable without referencing the story. \\
    \textbf{Correction:} \textit{It is cold to cut off contact with your family member.}

    \item \textbf{Bad RoT:} \textit{helped $\rightarrow$ It’s kind to help people.} \\
    \textbf{Reason:} Too vague. Needs more specificity. \\
    \textbf{Correction:} \textit{It is kind to help elderly people who are struggling with standing on a bus.}
\end{itemize}

\vspace{1em}
\noindent You don’t need to agree with the above examples. They are just illustrations. We want your own RoTs that reflect social norms in \textbf{Iran}.

\vspace{1em}
\noindent Now, please read the story first. Then click on a verb and type your judgments and actions. For each verb, you may write multiple RoTs. Once done, click the verb again to close it for convenience.
